# Supplementary material for: Kinetic pathways of coesite densification from metadynamics
Source: arXiv:2508.19716 ancillary file (2025-08-27)
Supplement: Supplementary file 1 [file Supplemental_Material.pdf]

# Kinetic pathways of coesite densification from metadynamics

## Supplemental Material

David Vrba and Roman Martoňák<sup>1</sup>

<sup>1</sup>*Department of Experimental Physics, Faculty of Mathematics, Physics and Informatics, Comenius University, Mlynská Dolina F2, 842 48 Bratislava, Slovakia*

This document provides additional details supporting the results presented in the main manuscript. It includes details of metadynamics simulations, shows the structures of coesite-IV and V, and provides some additional figures.

## Computational details

### Metadynamics simulations

Metadynamics[8] is an advanced enhanced sampling technique designed to overcome the limitations of plain molecular dynamics (MD), particularly its inefficiency in sampling rare events due to high free energy barriers. Effective sampling is achieved by introducing an artificial bias potential  $V_B$ , defined in terms of a few carefully chosen collective (CVs), modifying the potential energy of the system. During the simulation, Gaussian-shaped potentials are periodically deposited and added to the bias potential in the space of CVs, discouraging the system from revisiting previously explored regions. Deposition of potentials gradually fills the free energy wells, allowing the system to escape local minima and explore new configurations. The total bias potential can be written as:

$$V_B(\text{CVs}, t) = \sum_{t'=\tau_G, 2\tau_G \dots \leq t} W \exp \left( - \sum_{i=1}^d \frac{(s_i - s_i(t'))^2}{2\sigma_i^2} \right), \quad (1)$$

where  $W$  is the Gaussian height,  $\sigma_i$  is the Gaussian width and  $\tau_G$  is the frequency at which the Gaussian is deposited. In the limit, of  $t \rightarrow \infty$  method can be used to reconstruct an estimate of the underlying free energy surface (FES) as a function of the chosen CVs.

$$V_B(\text{CVs}, t \rightarrow \infty) = -F(s) + C. \quad (2)$$

For further background, we recommend the following review articles [17, 18].

In this work we used three CVs: global mean coordination number between Si and O atoms (CN), the volume per  $\text{SiO}_2$  unit and Si-Si coordination related CVs. The coordination number (CN) was computed using the `COORDINATION` keyword in PLUMED [21]. This implementation evaluates the number of contacts between two groups of atoms, in our case silicon and oxygen, based on switching function:

$$\text{CN}_{\text{SiO}} = \frac{1}{N_{\text{Si}}} \sum_{i \in \text{Si}} \sum_{j \in \text{O}} s_{ij}. \quad (3)$$

where the sums run over all Si and O pairs, and  $s_{ij}$  is the switching function defined as:

$$s_{ij}(r_{ij}) = \frac{1 - \left(\frac{r_{ij}-d_0}{r_0}\right)^n}{1 - \left(\frac{r_{ij}-d_0}{r_0}\right)^m}, \quad (4)$$

in case of  $m = 2n$  the switching function can be simplified further as:

$$s_{ij}(r_{ij}) = \frac{1}{1 + \left(\frac{r_{ij}-d_0}{r_0}\right)^n}, \quad (5)$$

Here,  $r_{ij}$  represents the distance between atoms  $i$  and  $j$ ,  $r_0$  represents the cutoff distance, and  $d_0$  represents a center-shift parameter.

The volume per  $\text{SiO}_2$  unit was computed using the `VOLUME` keyword in PLUMED [21]. This implementation evaluates the volume of the simulation box. This value was then divided by the number of  $\text{SiO}_2$  formula units.

### Metadynamics employing Si-O coordination number

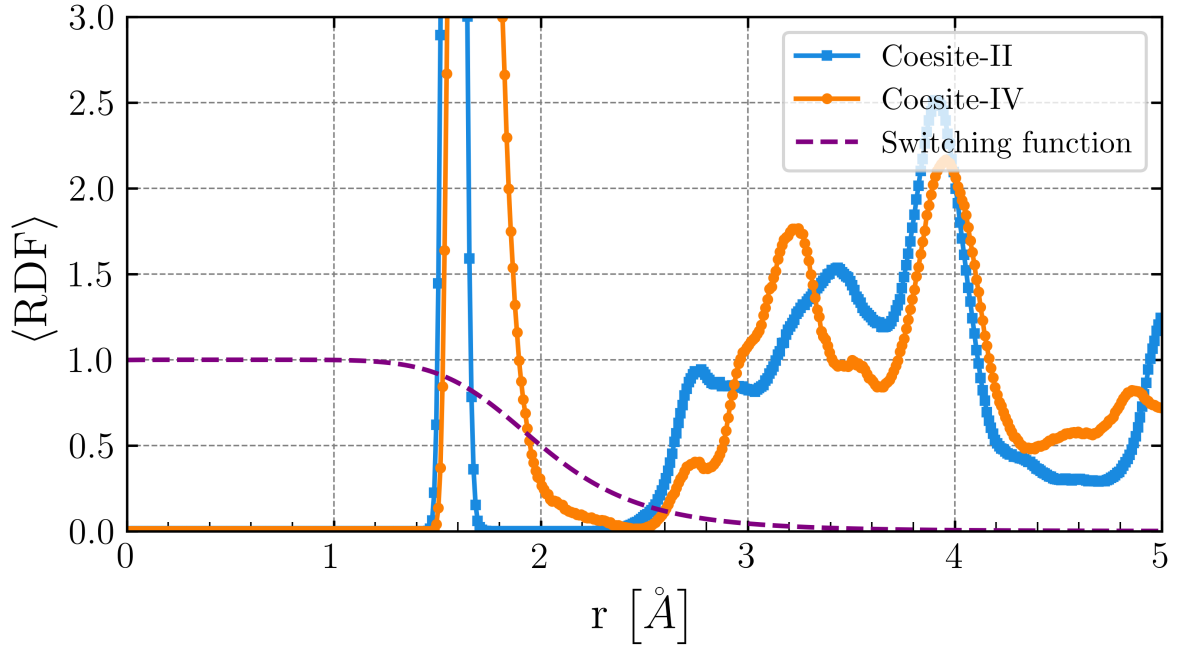

Supp. Mat. Figure 1: Si-O radial distribution functions of coesite-II and coesite-IV together with the switching function.

The switching function parameters were selected based on the comparison of radial distribution functions of coesite-II and coesite-IV (Supp. Mat. Fig.1). The switching function with parameters:  $d_0 = 0.5 \text{ Å}$ ,  $r_0 = 1.5 \text{ Å}$ ,  $n = 6$ , and  $m = 2n$  shown in the figure captures the difference in the Si-O coordination number between coesite-II and coesite-IV.

To improve computational efficiency, we used the neighbor list (NLIST) option with a neighbor list update stride of `NL_STRIDE` = 50 MD steps and a cutoff of `NL_CUTOFF` = 5 Å. The metadynamics parameters (Gaussian width and height) were chosen based on fluctuations of the CVs from plain MD simulations. All metadynamics runs using this  $\text{CN}_{\text{SiO}}$  and volume per  $\text{SiO}_2$  unit as CV, were performed with the same parameters:  $\sigma_{\text{CN}} = 0.03$ ,  $\sigma_{\text{Vol.}} = 0.06 \text{ Å}^3/\text{SiO}_2$ , a Gaussian height of 25 kJ/mol, and a Gaussian depositing frequency of 500 MD steps.

## Metadynamics employing Si-Si coordination-related CVs

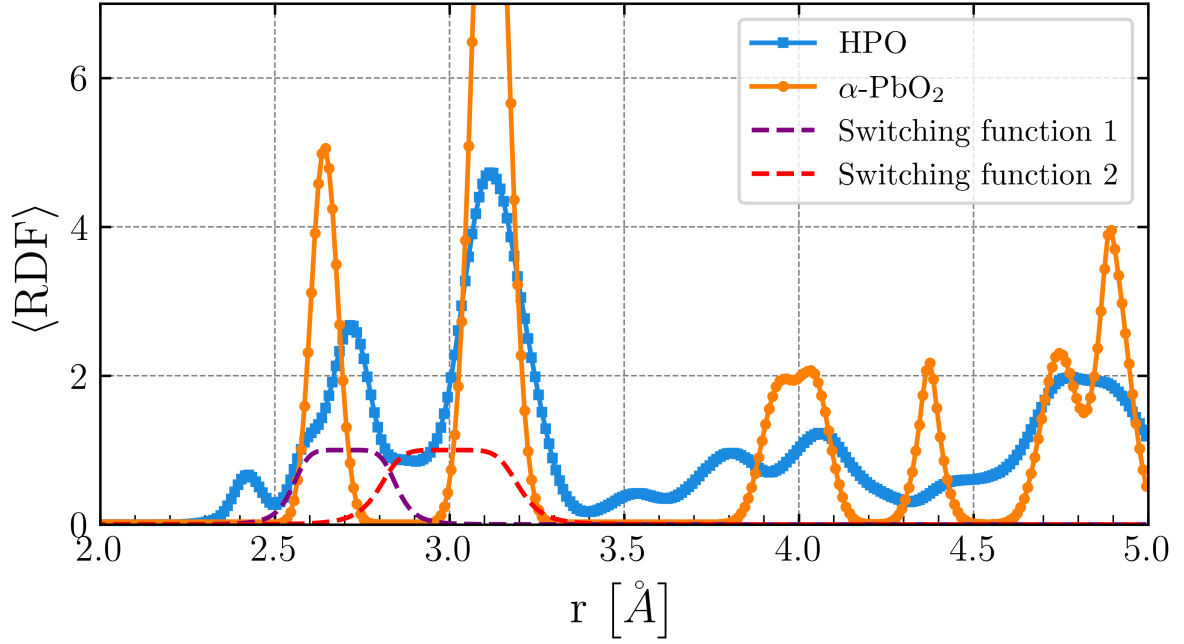

Supp. Mat. Figure 2: Si-Si radial distribution functions of the initial HPO phase and the  $\alpha$ -PbO<sub>2</sub> phase together with the two switching functions.

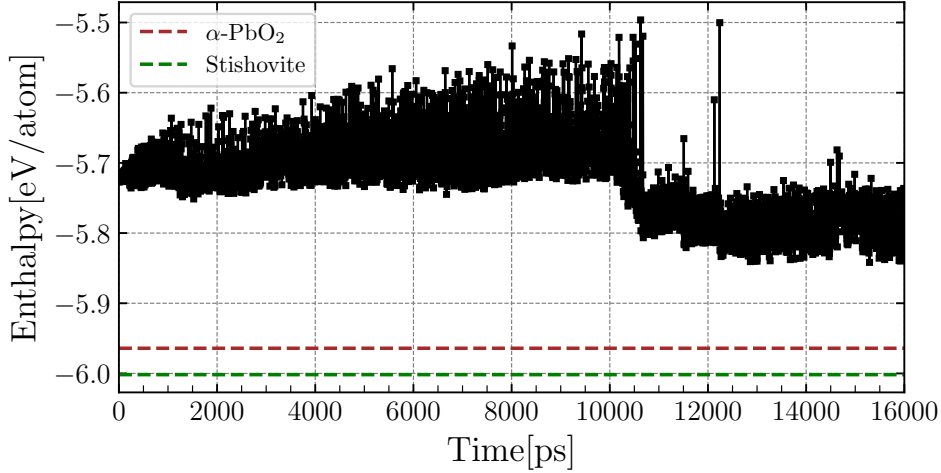

Supp. Mat. Figure 3: Evolution of the enthalpy during the metadynamics simulation employing Si-Si coordination-related CVs at  $p = 53$  GPa and  $T = 600$  K, starting from the initial HPO phase. The simulation showed that the enthalpy further decreases as the initially disordered chains gradually evolve towards the periodic  $2 \times 2$  pattern characteristic for the  $\alpha$ -PbO<sub>2</sub> phase.

In this case we deal with the problem of ordering of the Si atoms within the hcp sublattice of O atoms and therefore coordination Si-Si appears to be a good candidate to construct the CVs. Since one does not expect a substantial change of volume here, we use 2 Si-Si coordination related CVs and do not include the volume. The RDFs of the initial HPO phase and the  $\alpha$ -PbO<sub>2</sub>-like phase (to which the structure is expected to converge) are shown in Supp. Mat. Fig.2, together with the two switching functions we employed. These target the windows of

distances from 2.55 Å till 2.85 Å, and from 2.8 Å till 3.2 Å, respectively, where the RDFs of the two phases differ significantly. The two switching functions employed had the following parameters:

- Switching function 1:  $d_0 = 2.7$  Å,  $r_0 = 0.15$  Å,  $n = 6$ ,  $m = 12$
- Switching function 2:  $d_0 = 3.0$  Å,  $r_0 = 0.20$  Å,  $n = 6$ ,  $m = 12$

The same neighbor list settings were used as in the Si–O case. The metadynamics parameters were again derived from fluctuations observed in unbiased MD runs. Simulations using  $\text{CN}_{\text{SiSi}}$  were conducted with:  $\sigma_{\text{CN1}} = 0.375$ ,  $\sigma_{\text{CN2}} = 0.075$ , a Gaussian height of 75 kJ/mol, and PACE of 500 MD steps.

### ***Ab initio* calculations**

*Ab initio* calculations were carried out using the Vienna Ab initio Simulation Package (VASP) [27-30]. The Brillouin zone was sampled using a fully automatic  $\mathbf{k}$ -point mesh with a length parameter ( $R_k = 30$ ). The plane-wave energy cutoff was set to 560 eV (40% higher than the default VASP value) was selected based on convergence tests of the Pulay stress. We also used the energy convergence criterion of  $\text{EDIFF} = 10^{-6}$  eV and Gaussian smearing with a width of 0.05 eV. Structural relaxations were performed using the conjugate gradient algorithm, with a force convergence criterion of  $\text{EDIFFG} = -0.01$  eV/Å.

## Pathway to mixed and disordered structures

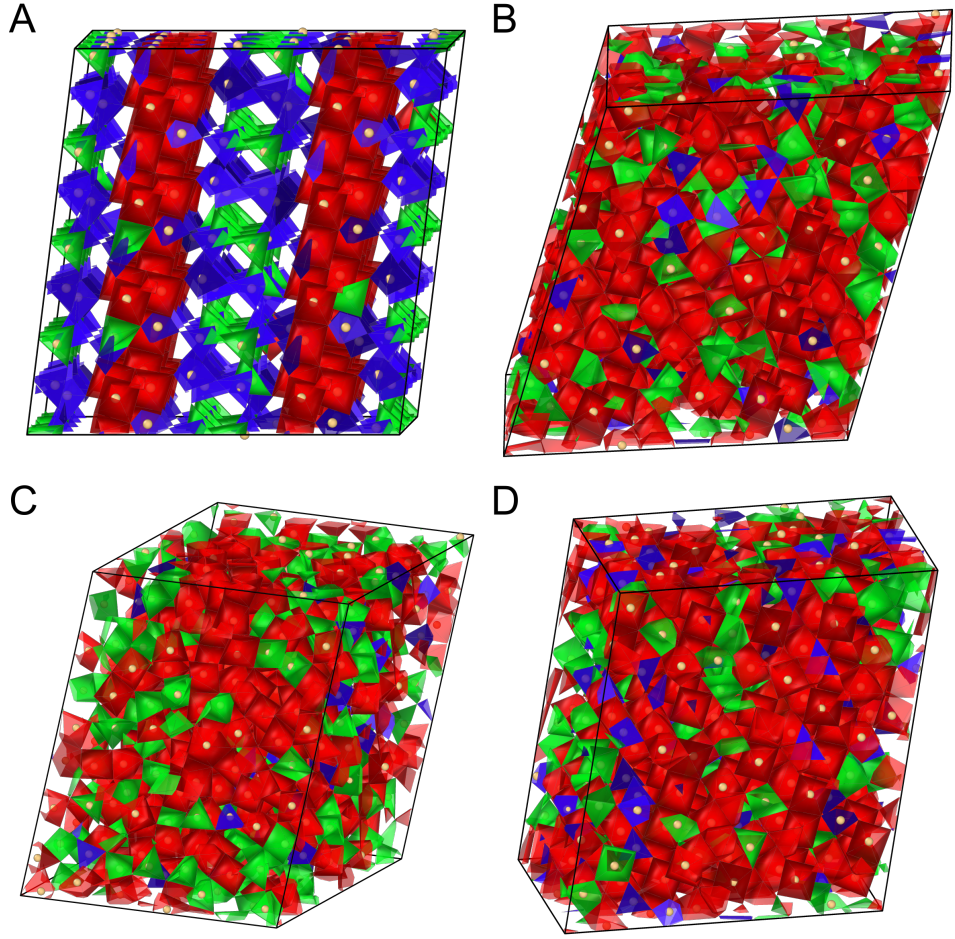

Supp. Mat. Figure 4: Structures of "2-chain" (**A**) and structures from three different simulations (**B,C,D**), which resulted in mixed or disordered phases. Si atoms are colored brown. Red, green and blue polyhedra represent 6-,5- and 4-coordinated Si atoms, respectively.

In two simulations at 300 K, the final structures appeared highly disordered, containing regions with defective crystalline parts. This failure in creating the crystalline structure is reflected in their elevated enthalpy compared to the rest of the runs (see the inset of Fig.9, black and green curves). In contrast, the remaining four simulations exhibited a distinct initial drop in enthalpy between 2.7 and 3.2 ns, indicative of the formation of an intermediate phase, which was consistently observed in all four simulations. We refer to this structure as the "2-chain", characterized by a specific arrangement of octahedra (see Supp. Mat. Fig.4 A). These systems maintained the "2-chain" structure for approximately 2.5 ns before gradually transforming to more mixed or disordered states (see Supp. Mat. Fig.4 B, C, D). Importantly, in all cases, the enthalpy remained substantially higher than that of the fully crystalline coesite-IV phase.

## Structures

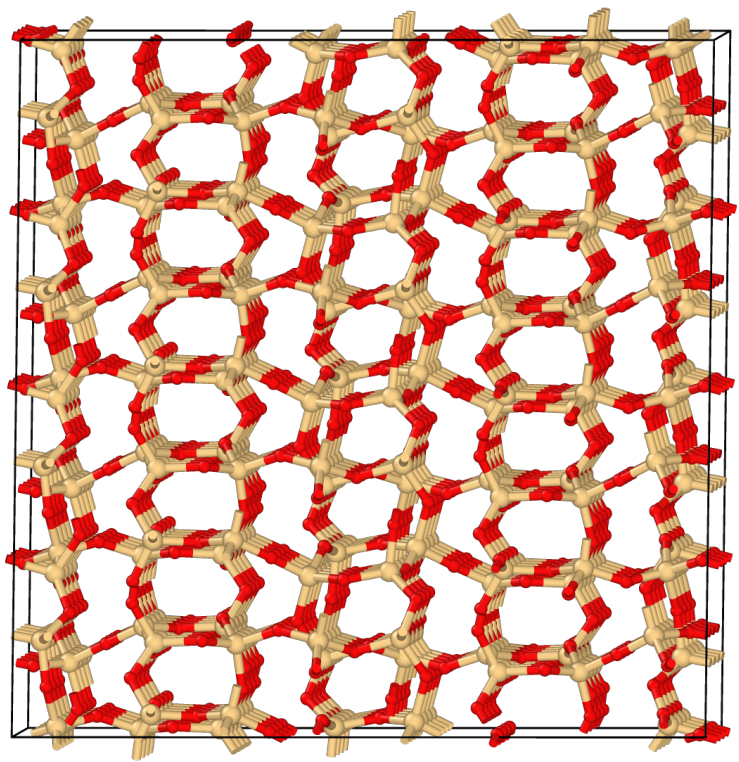

Supp. Mat. Figure 5: Initial structure of coesite-II (supercell  $4 \times 1 \times 4$  with 1536 atoms). Silicon atoms are colored brown and oxygen atoms are red.

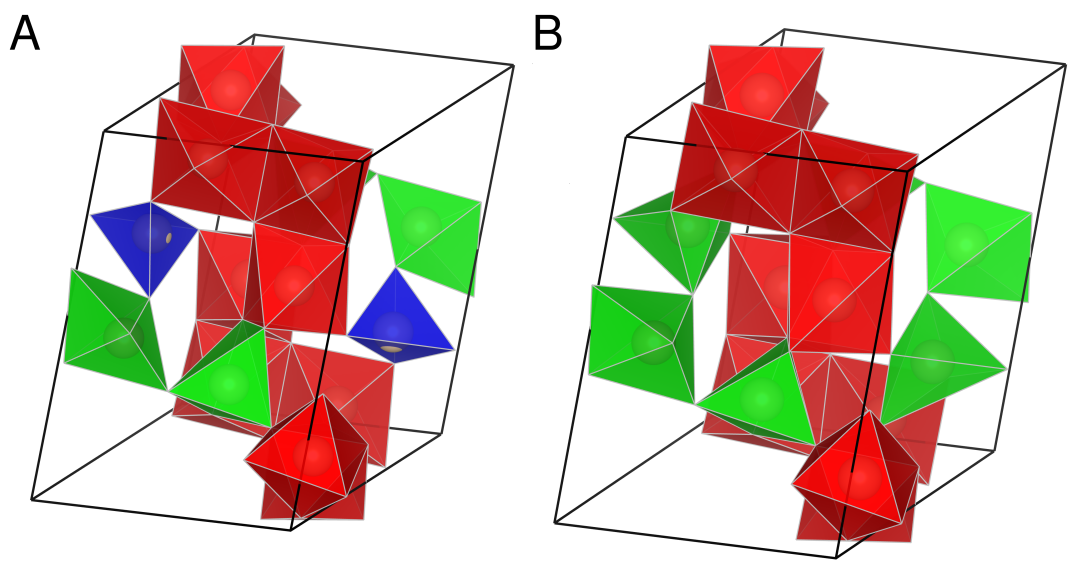

Supp. Mat. Figure 6: Structures of coesite-IV (**A**) and coesite-V (**B**) taken from Ref.[16]. Silicon atoms are colored brown. Red, blue and green polyhedra represent 6-, 5- and 4-coordinated Si atoms, respectively.
